# Supplementary material for: Unconventional anisotropic charge dynamics in bulk $1T$-TaS$_2$ induced by interlayer dimerization
Source: arXiv:2512.23883 source file (2026-09-11)
Supplement: Supplementary file 1 [file SM.pdf]

# Supplemental Material: Origin of insulating state in bulk $1T$-TaS$_2$ revealed by out-of-plane dimerization

Achyut Tiwari, Maxim Wenzel, Renjith Mathew Roy, Christian Prange, Bruno Gompf, and Martin Dressel
*1. Physikalisches Institut, Universität Stuttgart, Pfaffenwaldring 57, 70569 Stuttgart, Germany*
(Dated: December 29, 2025)

## S1. CRYSTAL STRUCTURE AND PHASE TRANSITIONS

$1T$-TaS$_2$ is a quasi-two-dimensional material composed of S-Ta-S, stacked sequentially via week van der Waals interactions. $1T$-TaS$_2$ crystallize in the P3/m1 space group with trigonal symmetry in high-temperature undistoreted phase. Each Ta atom is octahedrally coordinated by six sulfur (S) atoms, making perfecxt hexagonal plane in this phase.Upon cooling, the system undergoes a sequence of phase transitions: from an incommensurate metallic CDW phase (IC-CDW) above 350 K, to a nearly commensurate metallic CDW phase (NC-CDW) between 180 K and 350 K, and finally to a commensurate insulating CDW phase (C-CDW) below 180 K, and a broad thermal hysteresis with an intermediate triclinic phase (T-CDW) upon heating. The CDW phase Features a $\sqrt{13} \times \sqrt{13}$ periodic lattice distortion (PLD), where the entire crystalline plane is tiled by Star of David (SD) clusters, making it commensurate with the atomic lattice. This superlattice is typically rotated by 13.9° with respect to the atomic lattice. Star of David (SD) Clusters: Consist of 13 Ta atoms. The 12 outer Ta atoms contract towards the central Ta atom. The displacement of Ta atoms is accompanied by bulging of the S layers.

## S2. EXPERIMENTAL DETAILS

High-quality single crystals of $1T$-TaS$_2$ (HQ Graphene Co.) were grown by chemical vapor transport (CVT). Plate-like crystals with typical dimensions of $5 \times 2$ mm$^2$ and thickness $\sim 200, \mu$m were selected for transport and optical studies. Four-terminal resistivity was measured within the $ab$ plane and along the $c$ axis in a Physical Property Measurement System (PPMS, Quantum Design). For $c$-axis measurements, contacts were patterned on opposite faces to enforce uniaxial current flow and minimize geometric uncertainties.

To measure the $c$-axis optical response, the crystal cross-section was ion-beam polished (Leica cross-section polisher) to an optically flat surface (see inset of Fig.1 in main text). Infrared reflectivity at normal incidence was measured with a Bruker Vertex 80v spectrometer coupled to a Hyperion infrared microscope over 200–19,000, cm$^{-1}$ (24.8 meV–2.35 eV) from 300 K down to 10 K. Polarization-resolved reflectivity was obtained with $E \perp c$ ($ab$-plane response) and $E \parallel c$. Freshly evaporated gold mirror was used as reference for absolute reflectivity.

The complex optical conductivity was obtained from the measured reflectivity via Kramers–Kronig transformation. We applied Drude–Lorentz fits, utilizing the dc-conductivity obtained through transport measurements for extrapolations at lower frequencies, while x-ray scattering data were utilized to extrapolate the data in the high-frequency range.

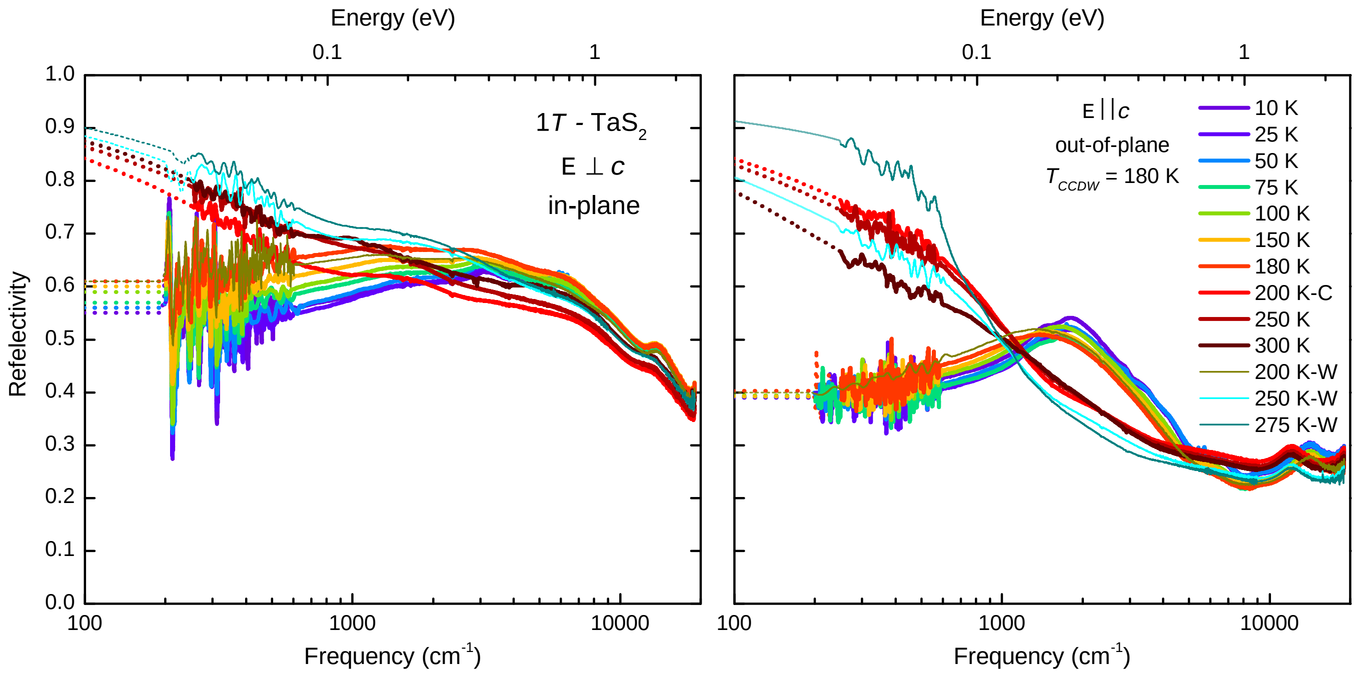


FIG. S1. Temperature-dependent reflectivity of a $1T$-$TaS_2$ single crystal measured with light polarized perpendicular to the $c$-axis ($ab$-plane response, left) and parallel to the $c$-axis (right) over a broad spectral range. Upon cooling, the reflectivity along both directions exhibits a marked suppression in the low-frequency region, signaling the opening of an energy gap at the commensurate charge-density-wave (CCDW) transition. Dotted lines indicate low-energy extrapolations based on Drude–Lorentz modeling. Thin lines correspond to spectra measured upon heating, highlighting the pronounced thermal hysteresis associated with the first-order nature of the metal–insulator transition.

## S3. DECOMPOSITION OF OPTICAL SPECTRA

We modeled the optical spectra using a Drude–Lorentz approach, in which the total dielectric function is expressed as the sum of itinerant carriers (Drude contribution) and bound electronic excitations (Lorentz oscillators):

$$\tilde{\varepsilon}(\omega) = \varepsilon_\infty - \frac{\omega_{p,\mathrm{Drude}}^2}{\omega^2 + i\omega/\tau_{\mathrm{Drude}}} + \sum_j \frac{\Omega_j^2}{\omega_{0,j}^2 - \omega^2 - i\omega\gamma_j}. \tag{S1}$$

where $\varepsilon_\infty$ denotes the high-energy contribution, $\omega_{p,\mathrm{Drude}}$ and $1/\tau_{\mathrm{Drude}}$ are the plasma frequency and scattering rate of the itinerant carriers, and $\omega_{0,j}$, $\Omega_j$, and $\gamma_j$ are the resonance frequency, oscillator strength, and linewidth of the $j^{\mathrm{th}}$ excitation, respectively. The complex optical conductivity $[\tilde{\sigma} = \sigma_1 + i\sigma_2]$ is obtained from:

$$\tilde{\sigma}(\omega) = -i\omega[\tilde{\varepsilon} - \varepsilon_\infty]/4\pi. \tag{S2}$$

The experimental optical spectra were fitted simultaneously to $\varepsilon_1(\omega)$, $\sigma_1(\omega)$, and the reflectivity by varying these parameters. In addition to electronic contributions, sharp Lorentz oscillators were included to account for phonon modes, which become prominent in the insulating C-CDW phase for in-plane polarization. Representative decompositions of the optical conductivity are shown in Fig. 2 (main text) for $T = 300$ K and 10 K, and in Fig. S2 for 200, 100, and 50 K.

In the NC-CDW phase, the in-plane ($E \perp c$) Drude contribution weakens upon cooling, while the out-of-plane ($E \parallel c$) Drude response strengthens, consistent with enhanced interlayer transport. Across $T_{CCDW}$, pronounced changes in the Lorentzian excitations and the emergence of sharp phonons in-plane highlight a redistribution of spectral weight and confirm that the electronic reconstruction is intrinsically three-dimensional.

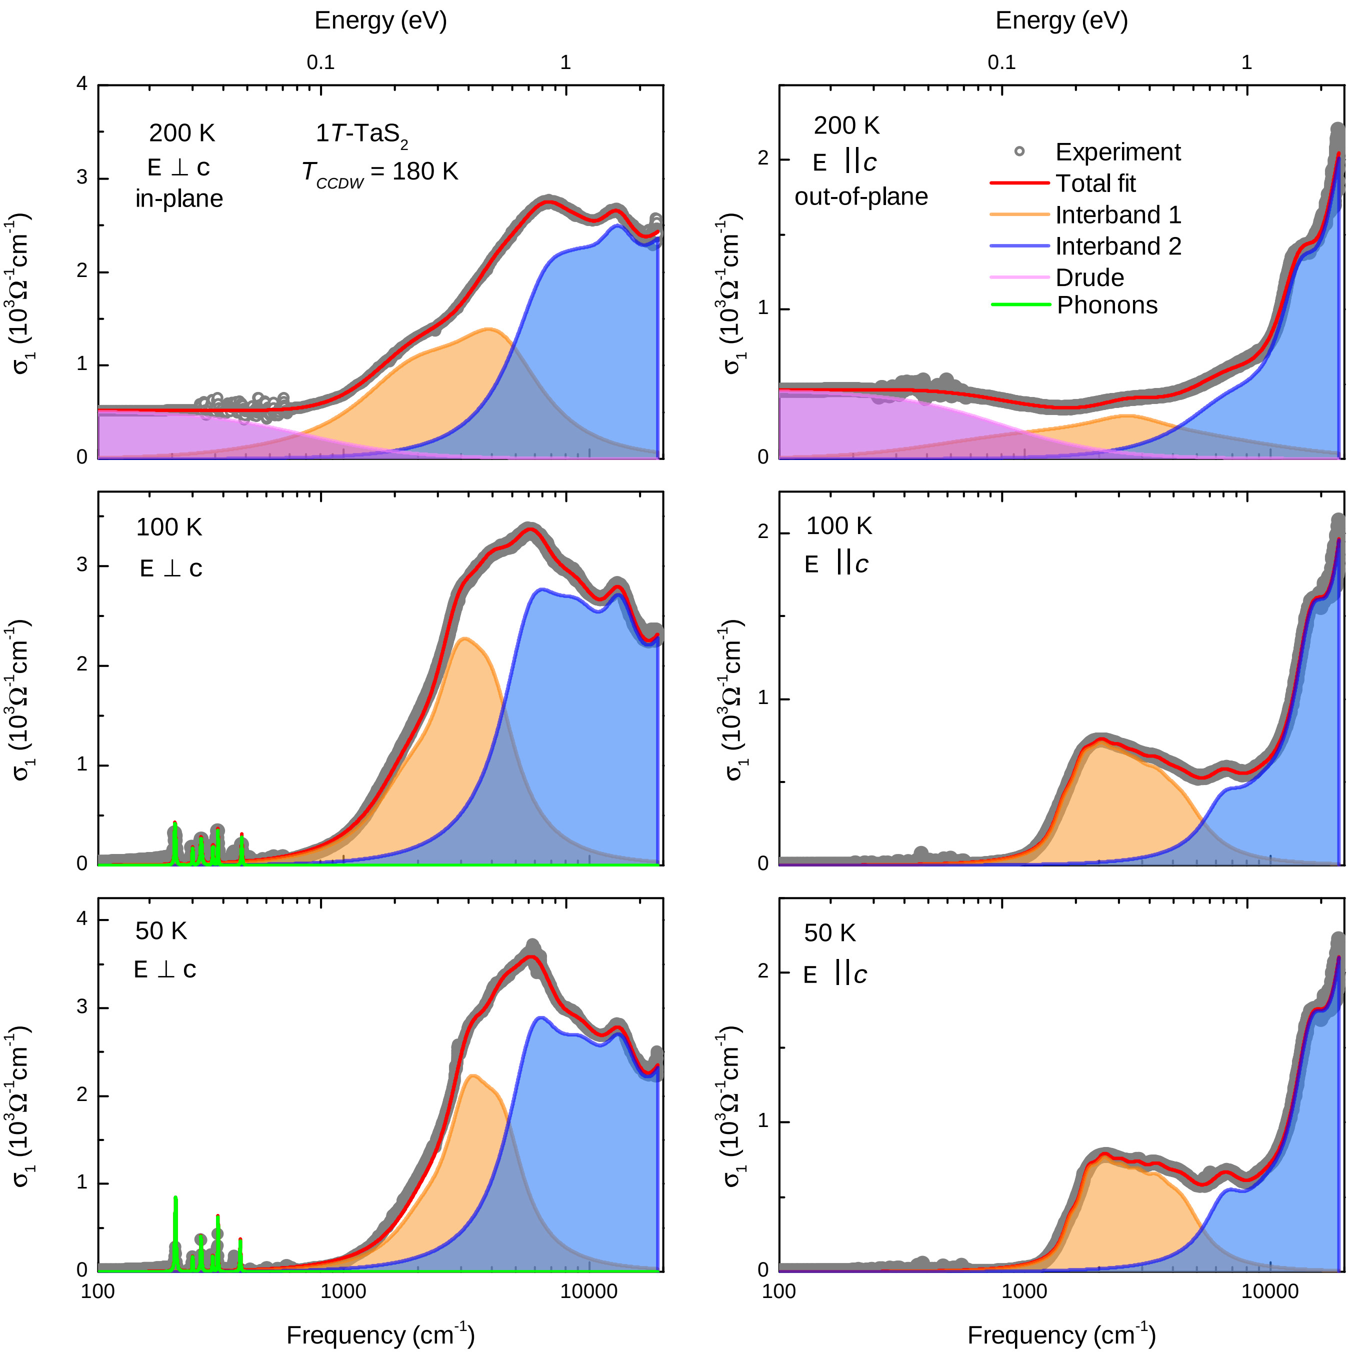


FIG. S2. Decomposition of the optical conductivity into a Drude component (magenta), mid-infrared interband transitions (orange), and high-energy interband transitions (blue) for the in-plane ($E \perp c$, left) and out-of-plane ($E \parallel c$, right) responses at 200 K, 100 K, and 50 K. The fits are obtained using the Drude–Lorentz approach, simultaneously fitting reflectivity, $\sigma_1$, and $\varepsilon_1$. Upon cooling, the in-plane Drude response weakens while the out-of-plane Drude response strengthens, highlighting the counterintuitive evolution of charge dynamics for layered materials. The pronounced redistribution of mid-infrared spectral weight in the low-temperature phase reflect a substantial reconstruction of the low-energy electronic structure across the CDW transition.

## S4. DFT CALCULATIONS

Density-functional-theory calculations were performed in the `Quantum Espresso` and `Wien2k` codes [1–4] within the generalized gradient approximation (GGA) employing the Perdew-Burke-Ernzerhof exchange-correlation functional [5]. Spin-orbit coupling was included in all calculations. Self-consistent calculations of the CCDW phase with $AL$ stacking [6], as presented in the main text, were converged on a $4 \times 4 \times 4$ $k$-mesh in `Quantum Espresso`, with the plane-wave energy cutoff and charge-density cutoff set to 30 Ry and 300 Ry, respectively. The optical conductivity was computed using the built-in `epsilon.x` module.

All other calculations presented in Section S5 were converged in `Wien2k` using the $k$-meshes summarized in Table S1. A Hubbard $U_{\mathrm{Ta}} = 2$ eV was added to the $3d$ Ta orbitals of the CCDW crystal structure from Ref. [7], using the LDA+$U$ (local density approximation) method with the FLL (fully localized limit) double-counting correction [see Fig.]. The optical conductivity tensors were calculated using the `OPTIC` module [8].

| structure/CIF-file | scf $k$-mesh | $k$-mesh for `OPTIC` |
|---|---|---|
| undistorted [9] | $13 \times 13 \times 5$ | $28 \times 28 \times 12$ |
| NCCDW [7] | | $13 \times 9 \times 15$ |
| CCDW [7] | $10 \times 7 \times 12$ | $18 \times 12 \times 21$ |
| $A$ stacking [10] | $10 \times 10 \times 10$ | $10 \times 10 \times 10$ |
| $L$ stacking [10] | $10 \times 10 \times 10$ | $10 \times 10 \times 10$ |
| $AL$ stacking [10] | $8 \times 8 \times 8$ | $8 \times 8 \times 8$ |

TABLE S1. $k$-point meshes used in the calculations with `Wien2k`.

Most CIF-files of the distorted structures have triclinic symmetry, in which the crystallographic $c$-axis does align with that of the actual measured single crystal. Therefore, the optical conductivity tensors obtained from `Wien2k` must be transformed from the triclinic basis to an orthonormal basis via [11]

$$\sigma_{\mathrm{orth}} = L \begin{pmatrix} \sigma_{xx} & \sigma_{xy} & \sigma_{xz} \\ \sigma_{yx} & \sigma_{yy} & \sigma_{yz} \\ \sigma_{zx} & \sigma_{zy} & \sigma_{zz} \end{pmatrix} L^{-1}, \tag{S3}$$

with

$$L = \begin{pmatrix} a & b\cos\gamma & c\cos\beta \\ 0 & b\sin\gamma & c\dfrac{\cos\alpha - \cos\beta\cos\gamma}{\sin\gamma} \\ 0 & 0 & c\sqrt{1 - \cos^2\beta - \left(\dfrac{\cos\alpha - \cos\beta\cos\gamma}{\sin\gamma}\right)^2} \end{pmatrix}. \tag{S4}$$

Here, $a, b, c, \alpha, \beta, \gamma$ are the triclinic lattice parameters.

## S5. ADDITIONAL COMPUTATIONAL RESULTS

DFT calculations of the undistorted structure ($T > 550$ K) [9] reveal metallic behavior, where interband transitions are absent below $\omega < 6000$ cm$^{-1}$ ($\sigma_{xx}$) and $\omega < 10000$ cm$^{-1}$ ($\sigma_{zz}$), as presented in Fig.S3(b).The presence of lower-energy interband transitions in the experimental optical conductivity at temperatures above $T_{\rm CCDW} = 190$ K [see Fig. 2 in the main text] indicates a significant reconstruction of the electronic band structure in both the incommensurate CDW phase (observed above $\sim 270$ K) and the nearly commensurate CDW (NCCDW) phase for 190 K $< T <$ 270 K.

Recent XRD studies suggest a domain-like star-of-David (SoD) type distortion in the NCCDW phase, whereas a uniform in-plane SoD distortion is observed in the CCDW phase. The stacking sequence in the CCDW phase was refined as $L$ stacking and was not reported to undergo significant changes entering the NCCDW state [7]. Using the refined lattice parameters from Ref. [7], we computed the band structures for the NCCDW and CCDW phases (Fig.). In the NCCDW phase, the calculated in-plane optical conductivity reproduces the experimental results remarkably well, while the out-of-plane conductivity deviates strongly from experiment.

While the density of states at the Fermi energy is slightly reduced, the calculations do not reproduce the insulating character in the CCDW phase. While the in-plane interband response matches well with the experimental observations, the calculated out-of-plane conductivity fails to reproduce the experimental observations, overall suggesting that 1$T$-$TaS_2$ does not adapt the $L$ stacking neither in the NCCDW nor in the CCDW phase. Since previous studies have suggested that the gap opening in the CCDW phase could be driven by electronic correlations, i.e., a Mott insulating state, we included a Hubbard $U = 2$ eV on the 3$d$ Ta orbitals. The resulting band structure shows almost no change (Fig.S3), consistent with other DFT studies and indicating that correlations alone cannot account for the gap opening.

Theoretical studies suggest that the gap opening in the CCDW phase is driven by interlayer stacking. Several out-of-plane structural modulations have been proposed, and we found the best agreement with the dimerized $AL$ stacking reported in Ref. [6], as discussed in the main text. Figure S4 presents the band structures and calculated optical conductivities for different stackings using the crystal structures from Ref. [10]. Notably, an insulating state is only obtained for the $AL$ stacking when using the modified Becke-Johnson (mBJ) exchange-correlation potential. For this configuration, the calculated optical conductivities closely match those obtained from the crystal structure in Ref. [6] [see Fig. 3 of the main text].

## S6. CALCULATION FOR DIFFRENT STACKING CONFIGURATIONS

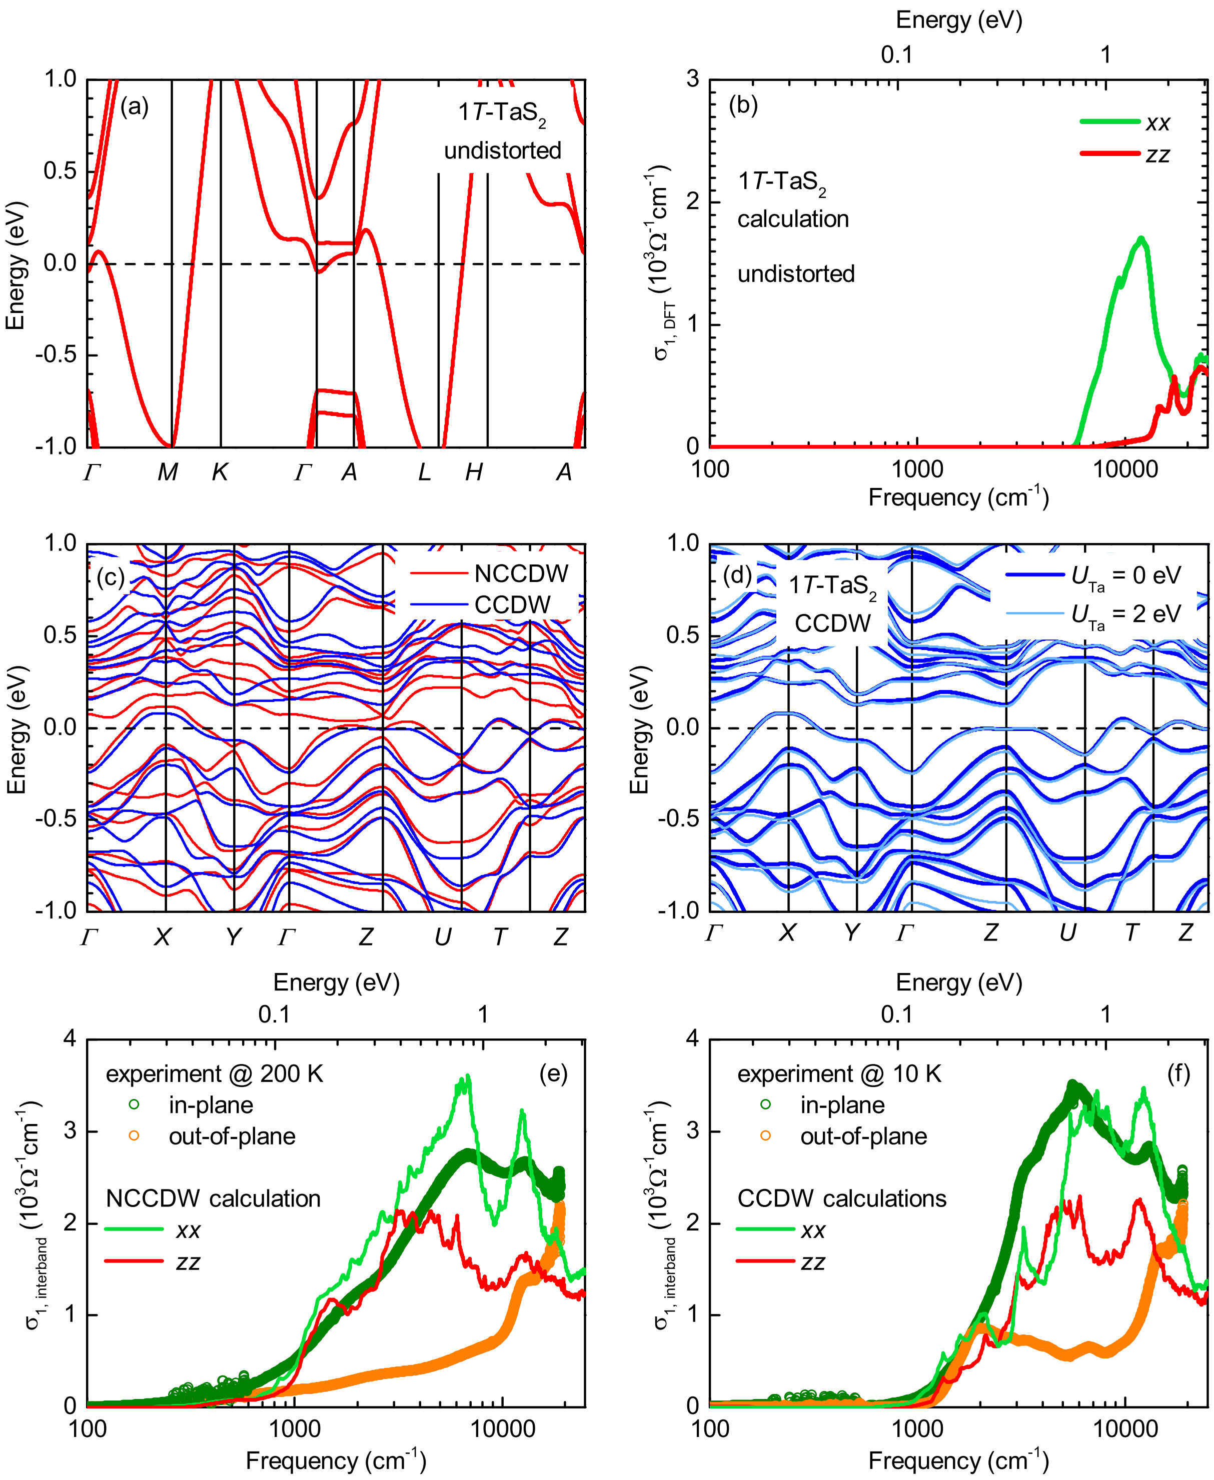


FIG. S3. (a, b) Calculated band structure and optical conductivity for undistorted phase. (c) Calculated band strucutre for NCCDW and CCDW phase. (d) Band structure for different Correlation values U. (e,f) Comparison of the measured real part of the optical conductivity, $\sigma_1(\omega)$ for in-plane and out-of-plane, with the optical response calculated from density-functional theory for the NCCDW and CDW phase.

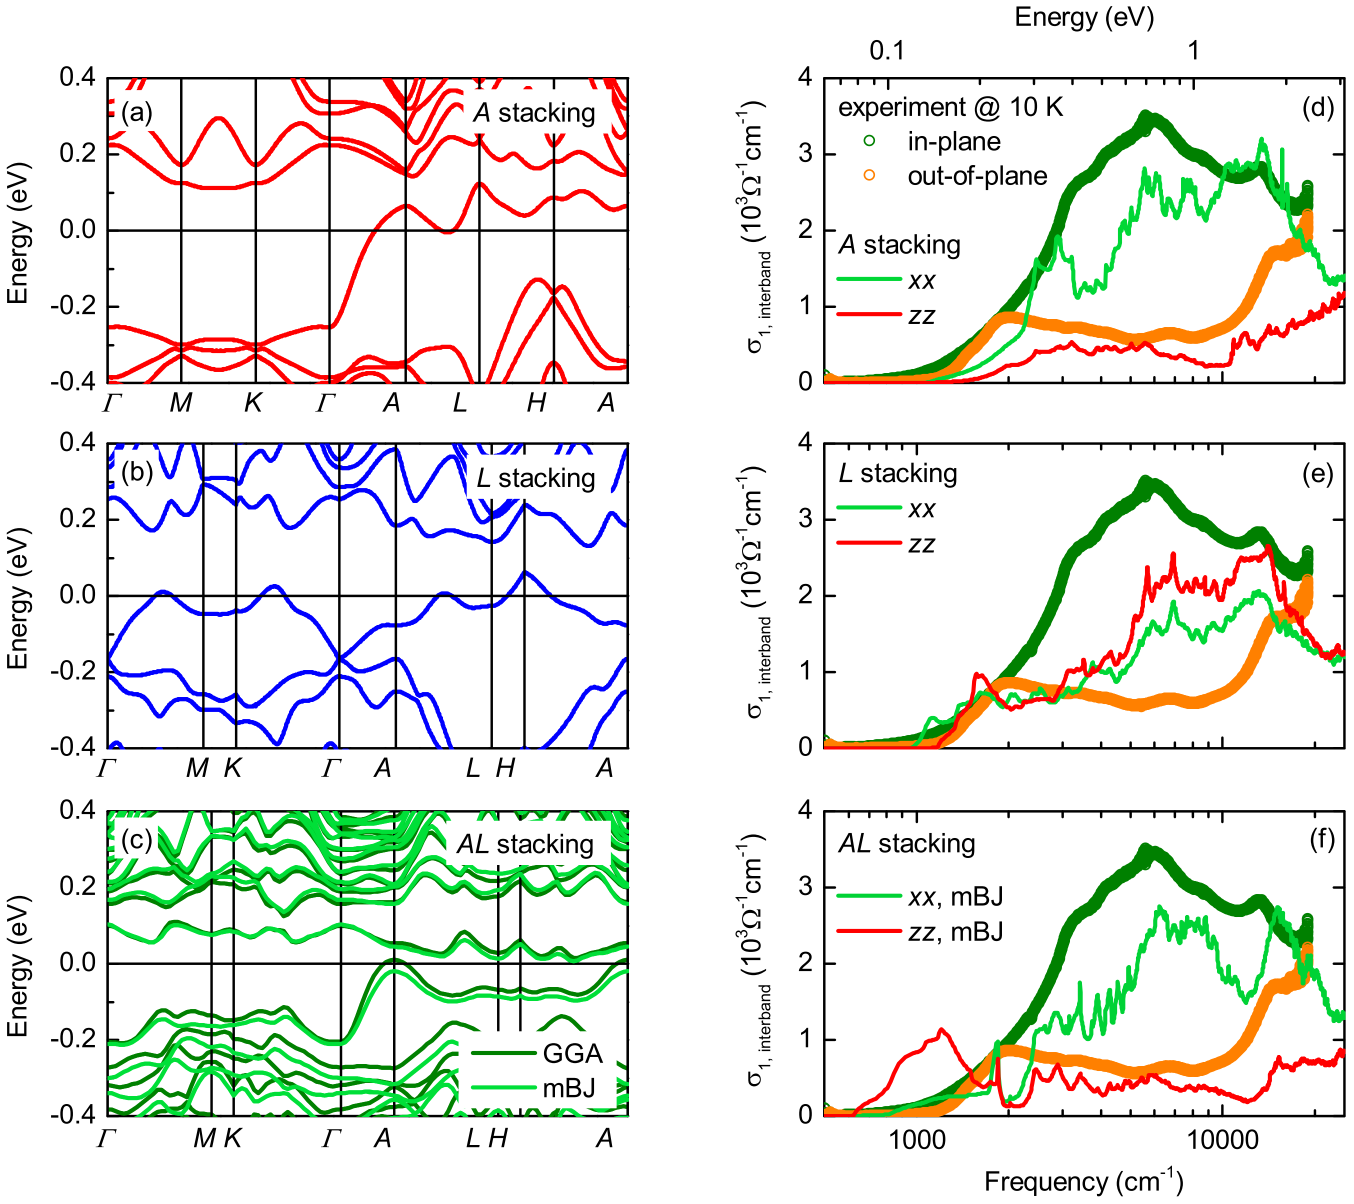


FIG. S4. (a, b, c) Calculated band structure for the low-temperature CCDW phase for A, L and AL stacking with the dashed horizontal highlights the gap at the Fermi level (d, e, f) Comparison of the measured real part of the optical conductivity, $\sigma_1(\omega)$, with the optical response calculated from density-functional theory for the A, L and AL-stacked commensurate CDW structure.

---


[1] P. Giannozzi, S. Baroni, N. Bonini, M. Calandra, R. Car, C. Cavazzoni, D. Ceresoli, G. L. Chiarotti, M. Cococcioni, I. Dabo, A. Dal Corso, S. de Gironcoli, S. Fabris, G. Fratesi, R. Gebauer, U. Gerstmann, C. Gougoussis, A. Kokalj, M. Lazzeri, L. Martin-Samos, N. Marzari, F. Mauri, R. Mazzarello, S. Paolini, A. Pasquarello, L. Paulatto, C. Sbraccia, S. Scandolo, G. Sclauzero, A. P. Seitsonen, A. Smogunov, P. Umari, and R. M. Wentzcovitch, QUANTUM ESPRESSO: a modular and open-source software project for quantum simulations of materials, J. Phys. Condens. Matter **21**, 395502 (2009).

[2] P. Giannozzi, O. Andreussi, T. Brumme, O. Bunau, M. Buongiorno Nardelli, M. Calandra, R. Car, C. Cavazzoni, D. Ceresoli, M. Cococcioni, N. Colonna, I. Carnimeo, A. Dal Corso, S. de Gironcoli, P. Delugas, R. A. DiStasio, A. Ferretti, A. Floris, G. Fratesi, G. Fugallo, R. Gebauer, U. Gerstmann, F. Giustino, T. Gorni, J. Jia, M. Kawamura, H.-Y. Ko, A. Kokalj, E. Küçükbenli, M. Lazzeri, M. Marsili, N. Marzari, F. Mauri, N. L. Nguyen, H.-V. Nguyen, A. Otero-de-la

Roza, L. Paulatto, S. Poncé, D. Rocca, R. Sabatini, B. Santra, M. Schlipf, A. P. Seitsonen, A. Smogunov, I. Timrov, T. Thonhauser, P. Umari, N. Vast, X. Wu, and S. Baroni, Advanced capabilities for materials modelling with Quantum ESPRESSO, J. Phys. Condens. Matter **29**, 465901 (2017).

[3] P. Blaha, K. Schwarz, G. Madsen, D. Kvasnicka, J. Luitz, R. Laskowski, F. Tran, and L. Marks, WIEN2k, An Augmented Plane Wave + Local Orbitals Program for Calculating Crystal Properties (Karlheinz Schwarz, Techn. Universität Wien, Austria), 2018. ISBN 3-9501031-1-2.

[4] P. Blaha, K. Schwarz, F. Tran, R. Laskowski, G. K. H. Madsen, and L. D. Marks, WIEN2k: An APW+lo program for calculating the properties of solids, J. Chem. Phys. **152**, 074101 (2020).

[5] J. P. Perdew, K. Burke, and M. Ernzerhof, Generalized Gradient Approximation Made Simple, Phys. Rev. Lett. **77**, 3865 (1996).

[6] Y. Wang, Z. Li, X. Luo, J. Gao, Y. Han, J. Jiang, J. Tang, H. Ju, T. Li, R. Lv, S. Cui, Y. Yang, Y. Sun, J. Zhu, X. Gao, W. Lu, Z. Sun, H. Xu, Y. Xiong, and L. Cao, Dualistic insulator states in 1T-$TaS_2$ crystals, Nat. Commun. **15**, 3425 (2024).

[7] V. Petkov, J. E. Peralta, B. Aoun, and Y. Ren, Atomic structure and Mott nature of the insulating charge density wave phase of 1T-$TaS_2$, J. Phys. Condens. Matter **34**, 345401 (2022).

[8] C. Ambrosch-Draxl and J. O. Sofo, Linear optical properties of solids within the full-potential linearized augmented planewave method, Comput. Phys. Commun. **175**, 1 (2006).

[9] K. Persson, Materials Data on $TaS_2$ (SG:164) by Materials Project (2014).

[10] T. Ritschel, H. Berger, and J. Geck, Stacking-driven gap formation in layered 1T-$TaS_2$, Phys. Rev. B **98**, 195134 (2018).

[11] I.-H. Suh, Y.-S. Park, and J.-G. Kim, *ORTHON*: transformation from triclinic axes and atomic coordinates to orthonormal ones, J. Appl. Crystallogr. **33**, 994 (2000).
